# Supplementary material for: GTNet:Guided Transformer Network for Detecting Human-Object Interactions
Source: arXiv:2108.00596 source file (2023-09-11)
Supplement: Supplementary file 1 [file GTNet_supplementary_materials.pdf]

# GTNet: Guided Transformer Network for Detecting Human-Object Interactions

## Supplementary Materials

Anonymous CVPR 2021 submission

Paper ID 4930

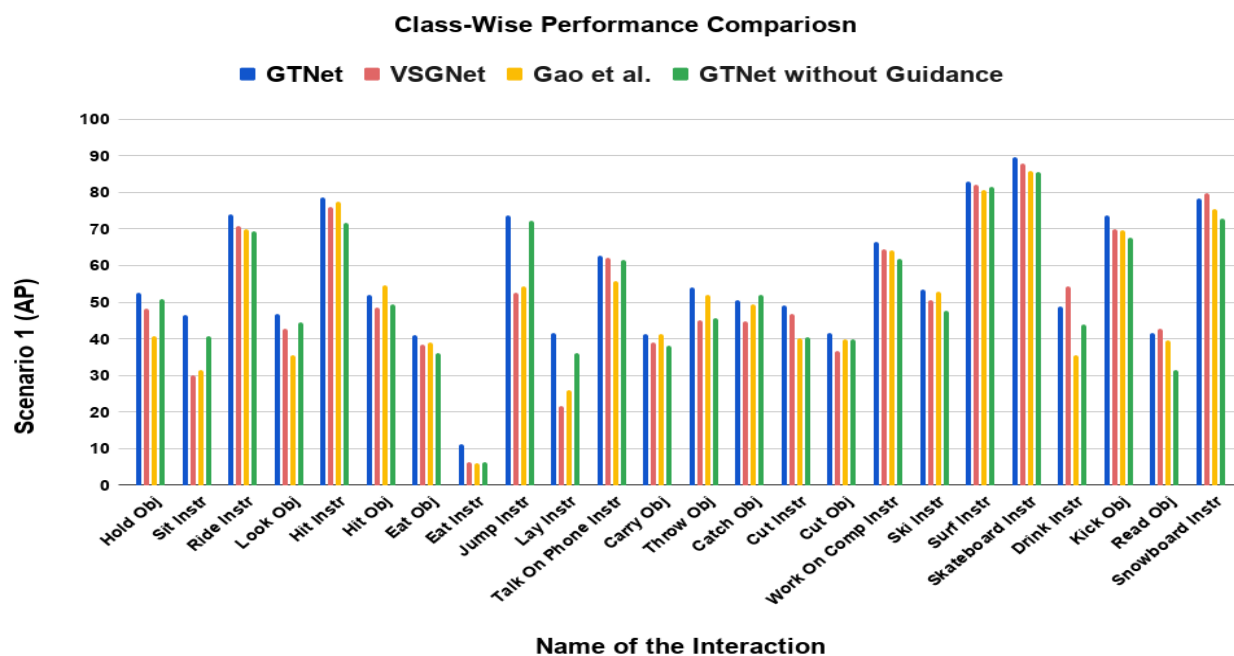

Figure 1. Class-wise performance comparison of GTNet with VSGNet [14] and Gao et al. [2] in V-COCO test set. We compare with the recent state of the art methods that reported class-wise AP values. Moreover, we also compare GTNet’s performance without the guidance mechanism to show the effect of Guidance Module. Obj is object and instr is instrument [5].

## 1. Introduction

GTNet proposes a guided self-attention based Transformer network to detect and localize interactions between humans and objects (HOI). This supplementary material includes in detailed comparisons with state of the art methods and additional experiments to validate different design choices for the proposed GTNet.

## 2. Performance Comparisons

**Class-wise Performance:** We compare GTNet’s class-wise performance in V-COCO [5] test set with VSGNet [13] and

Gao et al. [2]. We also compare our network’s performance without the guidance mechanism to demonstrate the effectiveness of the Guidance Module. Without the guidance mechanism, GTNet’s performance is close to the state of the art methods, and with its guidance mechanism it exceeds the recent methods in most of the classes. For a few classes (jump instr, lay instr) the improvement from the recent state of the art methods are more than 10 AP. Moreover, in a small number of classes, the object detectors perform badly. As a result the overall AP values are low in those classes. Eating utensils (instruments) are usually very small and not clearly visible in many images, so the object de-

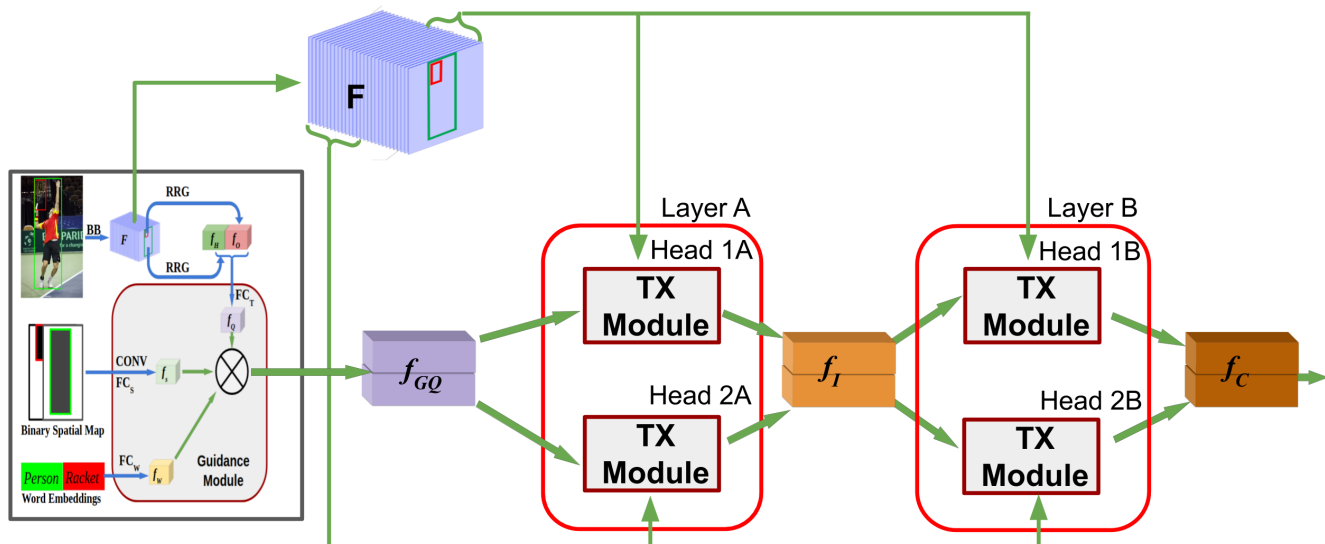

Figure 2. Stacking of TX Module. Two layers, two heads combination. Red colored boxes representing each layer. Each TX module inside the red box represents a head. Black box showing the input to the TX modules. Guided query vector  $f_{GQ}$  and input feature map  $F$  is divided into two equal parts to feed into two heads (Head 1A, Head 2A) in Layer A. The output of Layer A is concatenated ( $f_I$ ) and feed to the two heads (Head 1B, Head 2B) in Layer B. The final spatial context rich feature vector is the output of Layer B ( $f_C$ ) which will be fed to the Inference Module.

| Method               | Non-Rare    | Rare        | Full        |
|----------------------|-------------|-------------|-------------|
| iCAN [3]             | 17.7        | 11.3        | 16.3        |
| T. Wang et. al. [17] | 19.2        | 12.8        | 17.7        |
| Lin et. al [9]       | 20.6        | 14.6        | 19.2        |
| Li et al. [8]        | 20.3        | 15.5        | 19.2        |
| Wan et al. [15]      | 21.2        | 17.5        | 20.3        |
| H. Wang et al. [16]  | 21.1        | 20.7        | 21.0        |
| Liu et al. [10]      | 23.1        | 19.0        | 22.0        |
| Zhong et al. [18]    | <b>26.5</b> | 18.9        | 24.8        |
| DJ-RN [7]            | 24.6        | 20.6        | 23.7        |
| GTNet                | 26.3        | <b>20.9</b> | <b>25.0</b> |

Table 1. Performance comparison in HICO-DET in known object setting. The images are divided in Rare, Non-Rare, and Full Categories based on their numbers in the dataset. We only compare with the recent methods that reported their performance in known object setting

tectors miss them. Even with poor object detection results in eat instrument class, GTNet improves that class’s performance by  $\sim 6$  AP over recent state of the art methods.

**Performance in HICO-DET known object setting:** We compare GTNet’s performance in HICO-DET’s known object setting [1]. In this setting, for each HOI, AP is calculated only on the images that contains a certain object. For example, for the riding in a car HOI, AP is only calculated on the images that contains a car’s image. It is easier to achieve higher AP in this setting than the reported default

setting where all test images are considered for calculating AP [1]. Table 1 shows GTNet’s performance. GTNet performs better than the state of the art methods. GTNet’s performance significantly improves in Rare category (less than 10 training samples) from the default setting (17.6 to 20.9 AP). This shows GTNet has a higher false positive rate for the rare category, which can be fixed with higher number of training samples.

### 3. Additional Ablation Studies

**Stacking of TX Modules:** To get a better feature representation in the updated queries we stack multiple TX modules. Following [4], we use the concept of heads and layers.

Each layer is made up of  $H$  heads. The input to the first layer is  $f_{GQ}$ , the guided query. This input is split into  $H$  parts, one for each head. Similarly, the feature map  $F$  is split into  $H$  parts such that the input to each head is one part of  $F$  and one part of  $f_{GQ}$ . The input to each intermediate layer is the concatenated output of the previous layer and the feature map  $F$ . All layers get the same  $F$  but a modified query vector. We always use same number of heads in all the layers. Fig 2 illustrates an example of a configuration with two heads and two layers. We experiment with different combinations and find that two heads and two layers combination perform best in V-COCO test set (Table 2). Similarly, for HICO-DET we empirically choose a com-

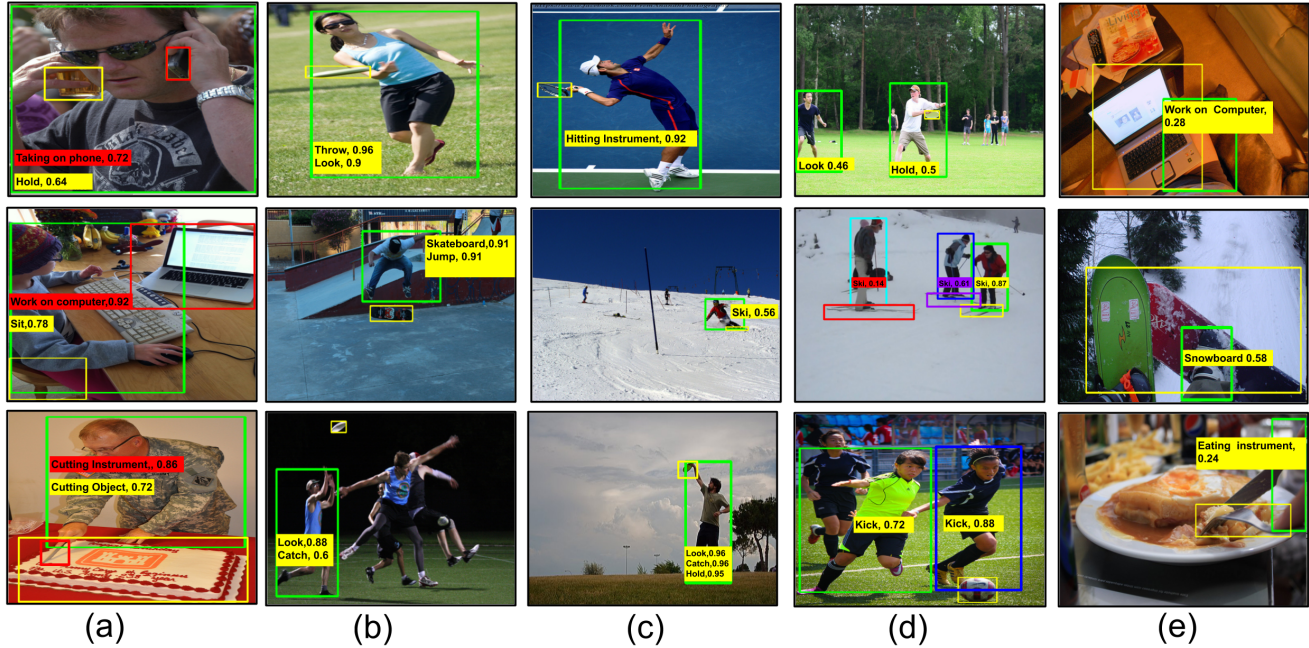

Figure 3. Visualized HOI detection results in V-COCO [5] test set. Each human bounding box includes predicted interaction labels for that human. Interaction labels and the bounding boxes of the interacting objects are in the same color. Each column represents a different situation: (a) a single human is interacting with multiple objects, (b) no contact between interacting human and object, (c) interacting object is small or not visible fully, (d) multiple humans are interacting with either same object or different objects, (e) interacting human is not fully present in the image.

| Layers→<br>Heads↓ | 1     | 2           | 3     |
|-------------------|-------|-------------|-------|
| 1                 | 56.09 | 55.92       | 55.79 |
| 2                 | 55.8  | <b>56.4</b> | 56.2  |
| 4                 | 56.24 | 55.8        | 55.62 |

Table 2. GTNet’s performance on V-COCO test set for different number of heads and layers.

| Backbone           | Scenario 1(mAP) |
|--------------------|-----------------|
| Vgg19 [11]         | 53.22           |
| Efficient Net [12] | 53.0            |
| Resnet-34 [6]      | 54.52           |
| Resnet-50 [6]      | 55.42           |
| Resnet-101 [6]     | 54.89           |
| Resnet-152 [6]     | <b>56.4</b>     |

Table 3. GTNet’s performance with different backbones. As can be seen, Resnet-152 achieves the best mAP in Scenario 1 of V-COCO test set.

combination of two heads and three layers. As can be seen, the network’s performance is not very sensitive to different combinations.

**Different Backbone Networks:** We test with different Convolutional Neural Networks(CNN) as our feature extractor backbone networks. Table 3 shows the performance of different backbones. We use Resnet-152 as our backbone as it achieves best result among different backbones.

**Visualized Detections:** In Fig. 3 we visualize few predicted HOIs by GTNet. Each column in the figure represents a different situation. GTNet performs pretty well across various situations. Moreover, as mentioned in the main paper, our network performs poorly when interacting human is not fully present in the image. This case is shown in column (e) in Fig. 3.

## References

- [1] Yu-Wei Chao, Yunfan Liu, Xieyang Liu, Huayi Zeng, and Jia Deng. Learning to detect human-object interactions. In *2018 IEEE winter conference on applications of computer vision (wacv)*, pages 381–389. IEEE, 2018. 2
- [2] Chen Gao, Jiarui Xu, Yuliang Zou, and Jia-Bin Huang. Drg: Dual relation graph for human-object interaction detection. *arXiv preprint arXiv:2008.11714*, 2020. 1
- [3] Chen Gao, Yuliang Zou, and Jia-Bin Huang. ican: Instance-centric attention network for human-object interaction detection. In *British Machine Vision Conference*, 2018. 2
- [4] Rohit Girdhar, Joao Carreira, Carl Doersch, and Andrew Zisserman. Video action transformer network. In *Proceedings of the IEEE Conference on Computer Vision and Pattern Recognition*, pages 244–253, 2019. 2
- [5] Saurabh Gupta and Jitendra Malik. Visual semantic role labeling. *arXiv preprint arXiv:1505.04474*, 2015. 1, 3
- [6] Kaiming He, Xiangyu Zhang, Shaoqing Ren, and Jian Sun. Deep residual learning for image recognition. In *Proceed-*

ings of the IEEE conference on computer vision and pattern recognition, pages 770–778, 2016. 3

[7] Yong-Lu Li, Xinpeng Liu, Han Lu, Shiyi Wang, Junqi Liu, Jiefeng Li, and Cewu Lu. Detailed 2d-3d joint representation for human-object interaction. In *Proceedings of the IEEE/CVF Conference on Computer Vision and Pattern Recognition*, pages 10166–10175, 2020. 2

[8] Yong-Lu Li, Siyuan Zhou, Xijie Huang, Liang Xu, Ze Ma, Hao-Shu Fang, Yanfeng Wang, and Cewu Lu. Transferable interactiveness knowledge for human-object interaction detection. In *Proceedings of the IEEE Conference on Computer Vision and Pattern Recognition*, pages 3585–3594, 2019. 2

[9] Xue Lin, Qi Zou, and Xixia Xu. Action-guided attention mining and relation reasoning network for human-object interaction detection. 2

[10] Y Liu, Q Chen, and A Zisserman. Amplifying key cues for human-object-interaction detection. *Lecture Notes in Computer Science*. 2

[11] Karen Simonyan and Andrew Zisserman. Very deep convolutional networks for large-scale image recognition. *arXiv preprint arXiv:1409.1556*, 2014. 3

[12] Mingxing Tan and Quoc V Le. Efficientnet: Rethinking model scaling for convolutional neural networks. *arXiv preprint arXiv:1905.11946*, 2019. 3

[13] Oytun Ulutan, ASM Iftekhar, and Bangalore S Manjunath. Vsgnet: Spatial attention network for detecting human object interactions using graph convolutions. In *Proceedings of the IEEE/CVF Conference on Computer Vision and Pattern Recognition*, pages 13617–13626, 2020. 1

[14] Oytun Ulutan, Swati Rallapalli, Mudhakar Srivatsa, Carlos Torres, and BS Manjunath. Actor conditioned attention maps for video action detection. In *The IEEE Winter Conference on Applications of Computer Vision*, pages 527–536, 2020. 1

[15] Bo Wan, Desen Zhou, Yongfei Liu, Rongjie Li, and Xuming He. Pose-aware multi-level feature network for human object interaction detection. In *Proceedings of the IEEE International Conference on Computer Vision*, pages 9469–9478, 2019. 2

[16] Hai Wang, Wei-shi Zheng, and Ling Yingbiao. Contextual heterogeneous graph network for human-object interaction detection. *arXiv preprint arXiv:2010.10001*, 2020. 2

[17] Tiancai Wang, Rao Muhammad Anwer, Muhammad Haris Khan, Fahad Shahbaz Khan, Yanwei Pang, Ling Shao, and Jorma Laaksonen. Deep contextual attention for human-object interaction detection. In *Proceedings of the IEEE International Conference on Computer Vision*, pages 5694–5702, 2019. 2

[18] Xubin Zhong, Changxing Ding, Xian Qu, and Dacheng Tao. Polysemy deciphering network for human-object interaction detection. In *Proc. Eur. Conf. Comput. Vis*, 2020. 2
